# Supplementary material for: BackdoorBench: A Comprehensive Benchmark of Backdoor Learning
Source: arXiv:2206.12654 source file (2022-10-19)
Supplement: Supplementary file 5 [file appendix_frequency_map.tex]

\subsubsection{Frequency salience map}

% Frequency saliency map (FSM) In addition to above two off-the-shelf visualization tools in the spatial domain, we also propose a novel visualization tool in the frequency domain. Inspired by
% the gradient-based visualization in the spatial domain, we aim to establish the connection between classification and image's frequency spectra. To this end, we utilize the transformation between the spatial and frequency domain, i.e., Discrete Fourier Transform (DFT), as well the chain rule of gradient, to formulate the Frequency saliency map, as follows:
% $$
% \frac{\partial t_c}{\partial F(u, v)}=\sum_x^{N-1} \sum_y^{N-1} \frac{\partial t_c}{\partial f(x, y)} \cdot \frac{\partial f(x, y)}{\partial F(u, v)}=\sum_x^{N-1} \sum_y^{N-1} \frac{\partial t_c}{\partial f(x, y)} \cdot e^{i 2 \pi\left(\frac{u x+v y}{N}\right)},
% $$
% \blue{
% where $f(x,y)$ denotes a sample in spatial domain, and $F(u,v)$ denotes the sample's frequency spectra; $\overline{y}$ denotes the class score for a sample $f(x,y)$; $g(x,y)$ denotes  the gradient of the class score with respect to the input sample. 
% }
\blue{
In this subsection, we provide a frequency visualization method, which can show the contribution of every Fourier basis to model classification. We denote $\vx_{j}\in \sR^{H\times W \times C}$ is the $j$th clean image of size $H\times W \times C$ and $\tilde{\vx}=\DFT(\vx)$ is the corresponding frequency spectrum with $\DFT$ being the channel-wise Discrete Fourier Transform (DFT) operator \cite{FFT}. Since the spatial domain can transform to frequency domain via Discrete Fourier Transform (DFT), we define $F:\mathbb{C}^{H\times W\times C}\rightarrow\sR^{S}$ as the corresponding classifier in the frequency domain, which means
\begin{equation}
\label{DFT_f}
%\tilde{f} = f \circ \IDFT, 
F(\tilde{\vx}) = f(\vx) = f\big( \IDFT(\tilde{\vx}) \big), 
\end{equation}
where $\IDFT$ is the channel-wise Inverse Discrete Fourier Transform (IDFT) operator, which means $\IDFT(\tilde{x})=\sum_{h=0}^{H-1}\sum_{w=0}^{W-1}\tilde{x}(h,w)e^{-2\pi i(\frac{uh}{H}+\frac{vw}{W})}$.

Inspired by the saliency map in the RGB space, % the gradient-based ConvNet visualization methods, 
we intend to establish the connection between model prediction and image’s frequency spectrum by the norm of gradient. According to the chain's rule, we can estimate the gradient by the equation ~\ref{fre_equation},
\begin{equation}
    \begin{split}
    \gG_s(u,v,c)=\frac{\partial F_s(\tilde{\vx})}{\partial \tilde{\vx}(u,v,c)} &=
    \sum_{h=0}^{H-1}\sum_{w=0}^{W-1}\sum_{c'=0}^{C}\frac{\partial f_s(\vx)}{\partial \vx(h,w,c')} \cdot \frac{\partial \vx(h,w,c')}{\partial \tilde{\vx}(u,v,c)} \\
    &= 
    \sum_{h=0}^{H-1}\sum_{w=0}^{W-1}\frac{\partial f_s(\vx)}{\partial \vx(h,w,c)} e^{2\pi i(\frac{uh}{H}+\frac{vw}{W})}, 
    \end{split}
\end{equation}
where $f_s$ means the logit output of the model $f$ for the $s$-th label.}

\blue{
The visualization results of frequency have shown in Figure ~\ref{frequency map}, in which low-frequency components are shifted into the center regions while high-frequency components are distributed in surrounding regions. The first column displays some poisoned samples in spatial domain, such as BadNet, Blended, SSBA, WaNet, and LF. The second column shows the contribution of different frequency basis to backdoor model classification. It can be seen that most backdoor models pay attention to high-frequency regions, while LF attack make the model more concentrate on low-frequency regions. Besides, we are able to see obvious difference between SSBA and WaNet in Frequency domain, even though their spatial images are hard to distinguish. Hence, it is possible to use this visualization method to detect backdoors.}

\blue{
The rest of columns show the contribution of frequency basis to various defense models. For example, when the poisoned image was inputted in a BadNet model, the contribution of some high-frequency regions is huge. However, once FT worked on this backdoor model, the low-frequency regions regain the attention from the model. This phenomenon is consistent with Figure ~\ref{2-attack-asr-preact}, which shows that FT is able to remove backdoors embedded by BadNet and WaNet effectively. We intend to explore more properties through the perspective of frequency domain.
}

\begin{figure}[!ht]
    \centering
    \includegraphics[width=\textwidth]{figs_appendix/cifar10_frequency.pdf}
    % \vspace{-0.7em}
    \caption{\blue{Frequency visualization of regions which contribute to model classification under different attack methods and defense methods with PreAct-ResNet18 and 10\% poisoning rate on CIFAR-10.}}
    % \vspace{-1.6em}
    \label{frequency map}
\end{figure}
