# Supplementary material for: BackdoorBench: A Comprehensive Benchmark of Backdoor Learning
Source: arXiv:2206.12654 source file (2022-10-19)
Supplement: Supplementary file 7 [file appendix_memory_forget.tex]

\subsection{\blue{Analysis of backdoor forgetting}}
\label{appendix: subsec backdoor forgetting}

\comment{
\paragraph{Memorization} 

In this part, we utilize membership inference attack to explore the memorization of backdoored models. Different from the traditional settings of membership inference, we assume shadow models have the same performance as target models, \ie, backdoored models in our benchmark.

In our experiment, the membership inference attack model has one hidden layer with 64 neurons. Both the training dataset $D_{attack\_train}$ and the testing $D_{attack\_test}$ consist of four parts, which are clean samples in backdoored model's training dataset, poisoned samples in backdoored model's training dataset, clean samples out backdoored model's training dataset, and poison samples out backdoored model's training dataset. Indeed, the clean samples out backdoored model's training dataset come from original test dataset which was used to compute a backdoored model’s accuracy. In the same way, the poison samples out backdoored model's training dataset come from original poisoned test dataset which was used to compute a backdoored model’s ASR. However, $D_{attack\_train}$ and $D_{attack\_test}$ are different in the number of samples. We will display the detail of datasets in the experiment results.

In the experiment results, we mainly exhibit the memorization of the backdoored model trained on CIFAR-10 with PreactResNet18 backbone. The poison ratio is 10\%. The specific information of training and testing dataset is shown in Table ~\ref{mem-dataset}. Besides, we provide the inference accuracy of two backdoored models in Table ~\ref{mem-result}, which displays the accuracy of clean samples and poisoned samples respectively.

From the results, we discover that poisoned samples are more easily to be remembered than clean samples, even though the number of poisoned samples are much smaller than clean samples. This is probably due to the complication of trigger is simpler. 

\begin{table}
\centering
\caption{The detail of training and testing dataset on CIFAR-10 }\label{mem-dataset}
\begin{tabular}{|p{2cm}<{\centering}|p{2cm}<{\centering}|p{2cm}<{\centering}|p{2cm}<{\centering}|p{2cm}<{\centering}|}
\hline
 Dataset & clean\_in & poison\_in & clean\_out & poison\_out\\
\hline
Training  & 45000 & 5000 & 5000 & 4500\\
\hline
Testing & 5000 & 5000 & 5000 & 4500\\
\hline
\end{tabular}
\end{table}

\begin{table}
\centering
\caption{The result of memorization of BadNet and Blended backdoor attack}\label{mem-result}
\begin{tabular}{|p{4cm}<{\centering}|p{4cm}<{\centering}|p{4cm}<{\centering}|}
\hline
Backdoor Model  & inference accuracy of poisoned samples & inference accuracy of clean samples\\
\hline
BadNet  & 0.6 & 0.55\\
\hline
Blended & 0.59 & 0.56\\
\hline
\end{tabular}
\end{table}
}

%\paragraph{Forgetting}

From the above analysis about the quick learning of backdoor in Section \ref{appendix: sec quick learning}, we get one impression that the backdoored model memorizes the poisoned samples quickly and stably. 
To obtain more insights about the inner mechanism of backdoor learning, we adopt the concept of \textit{forgetting event} \cite{forgetting} to characterize the learning dynamics during the training process. Specifically, one forgetting event is recorded when a correctly predicted training sample at the current epoch is incorrectly predicted at the next epoch. 
Formally, given a training sample $(\mathbf{x},y)$, where $\mathbf{x}$ is input feature, $y$ is ground-truth label. 
If $\mathbf{x}$ is correctly predicted at the epoch $t$, \textit{i.e.}, $f_{\theta^t}(\mathbf{x})=y$, but is misclassified at epoch $t+1$, \textit{i.e.}, $f_{\theta^{t+1}}(\mathbf{x})\neq y$, where $f$ denotes the model and $\theta^t,\theta^{t+1}$ are model parameters at the epoch $t$ and $t+1$, then a forgetting event is recorded for this sample.

Specifically, we count the number of forgetting events for clean and poisoned training samples, respectively, on CIFAR-10 with Preact-ResNet18 backbone. 
The distributions of forgetting events of clean and poisoned samples are shown in Figure \ref{app:forget}. 
The results show that: 
\begin{itemize}
\item  The forgetting events of clean training samples follow an exponential distribution, and are similar among different cases. 
\item For poisoned training samples: \textbf{1)} when the poisoning ratio is low (\eg, 0.1\%, 0.5\%), the forgetting numbers of poisoned samples are often larger than those of clean samples; \textbf{2)} when the poisoning ratio is high (\eg, 5\%, 10\%), the forgetting numbers of poisoned samples are often smaller than those of clean samples.
\end{itemize}
The above observations are compatible with our high-level observation that the backdoor attack with higher poisoning ratios could quickly learn the stable mapping from the poisoned samples to the target class. Moreover, the forgetting event provides a fine-grained tool to analyze the contribution of each individual training sample, which could facilitate the development of more advanced backdoor attack and defense methods.

\begin{figure}[!ht]
    \centering
    \includegraphics[width=0.9\textwidth]{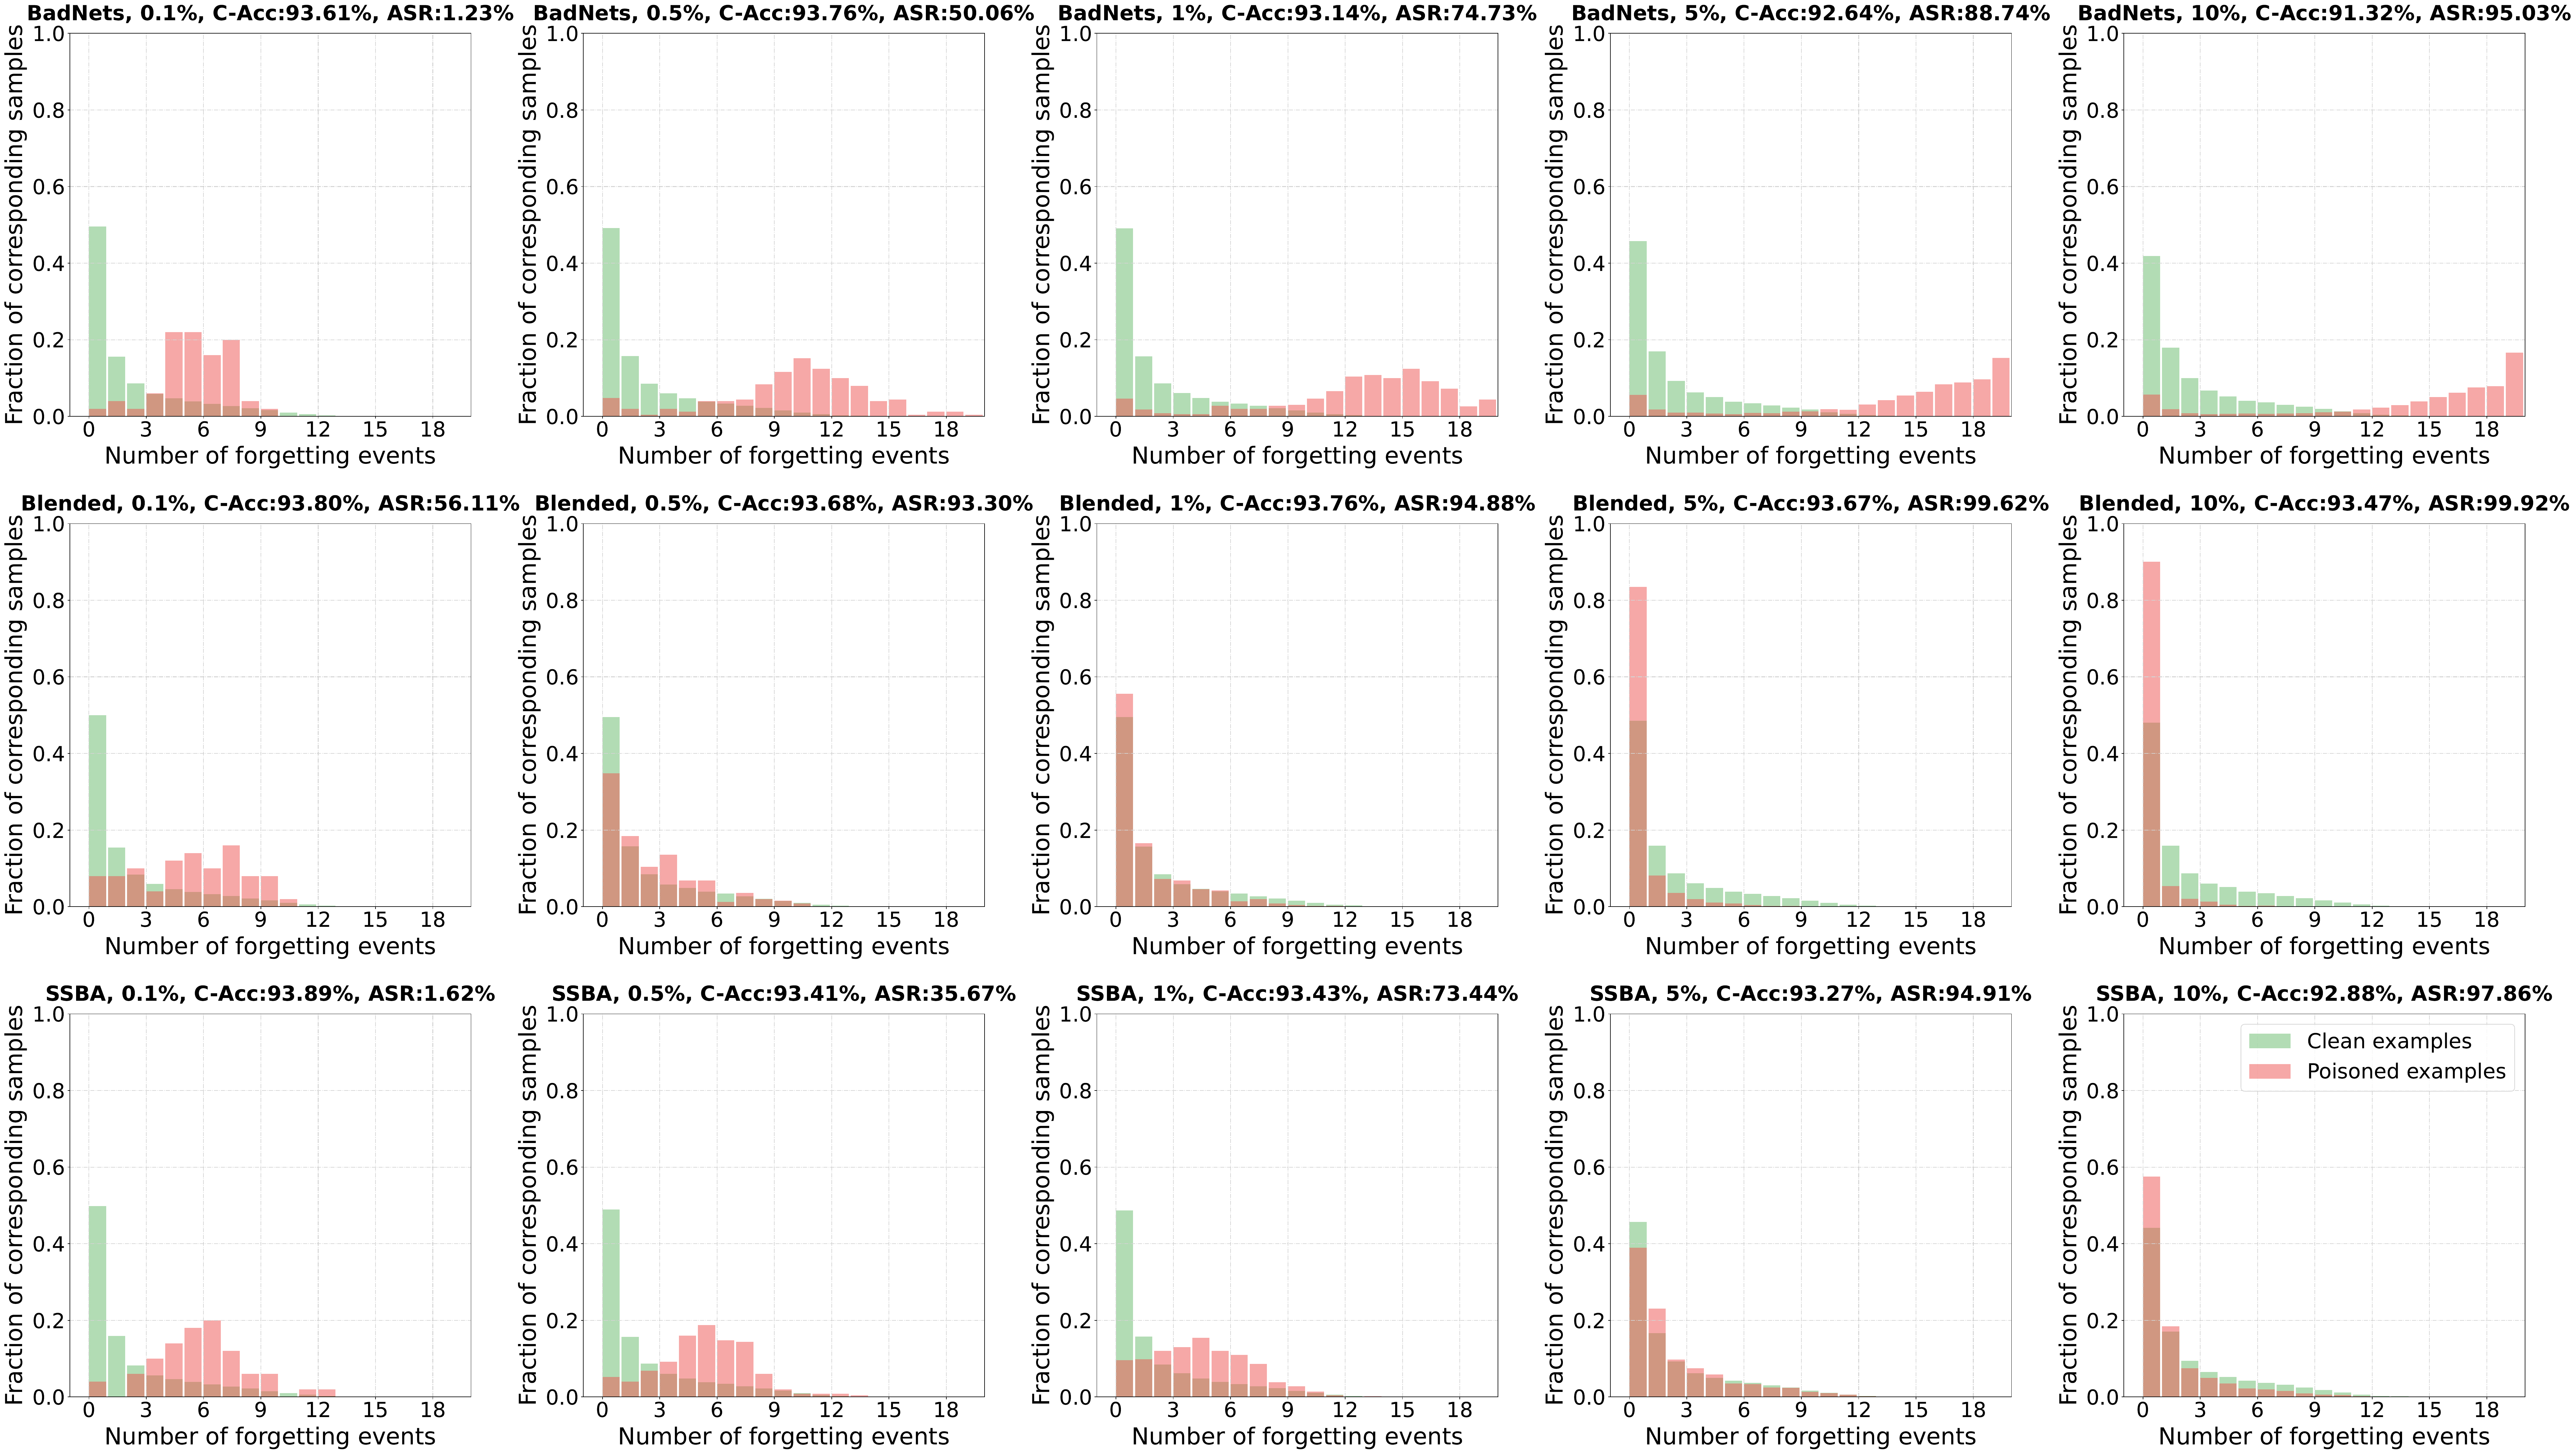}
    % \vspace{-0.7em}
    \caption{\blue{Distributions of forgetting events of clean training examples and poisoned examples in CIFAR-10 with Preact-Resnet18 backbone.}}
    % \vspace{-1.6em}
    \label{app:forget}
\end{figure}
