# Supplementary material for: BackdoorBench: A Comprehensive Benchmark of Backdoor Learning
Source: arXiv:2206.12654 source file (2022-10-19)
Supplement: Supplementary file 10 [file appendix_stable.tex]

\subsection{Stability of the poisoning ratio experiment}
\blue{
In this subsection, we mainly test the stability of poisoning ratio experiment. With ragard to the randomness due to weight initialization and some methods'mechanisms, we conducted relevant randomization experiments to test the stability of the experimental results.}

\paragraph{Experimental setting}
\blue{
We set a random seed in the code, which can ensure that the network initialization and mini batch training are fixed under the condition that the random seed is unchanged, that is, the uniqueness of the experimental results can be guaranteed. We use five different random seeds for each backdoor attack, backdoor defense, and poisoning ratio. We plotted the mean of each experiment and the error bar obtained according to the standard deviation.}

\begin{figure}[!ht]
    \centering
    \includegraphics[width=\textwidth]{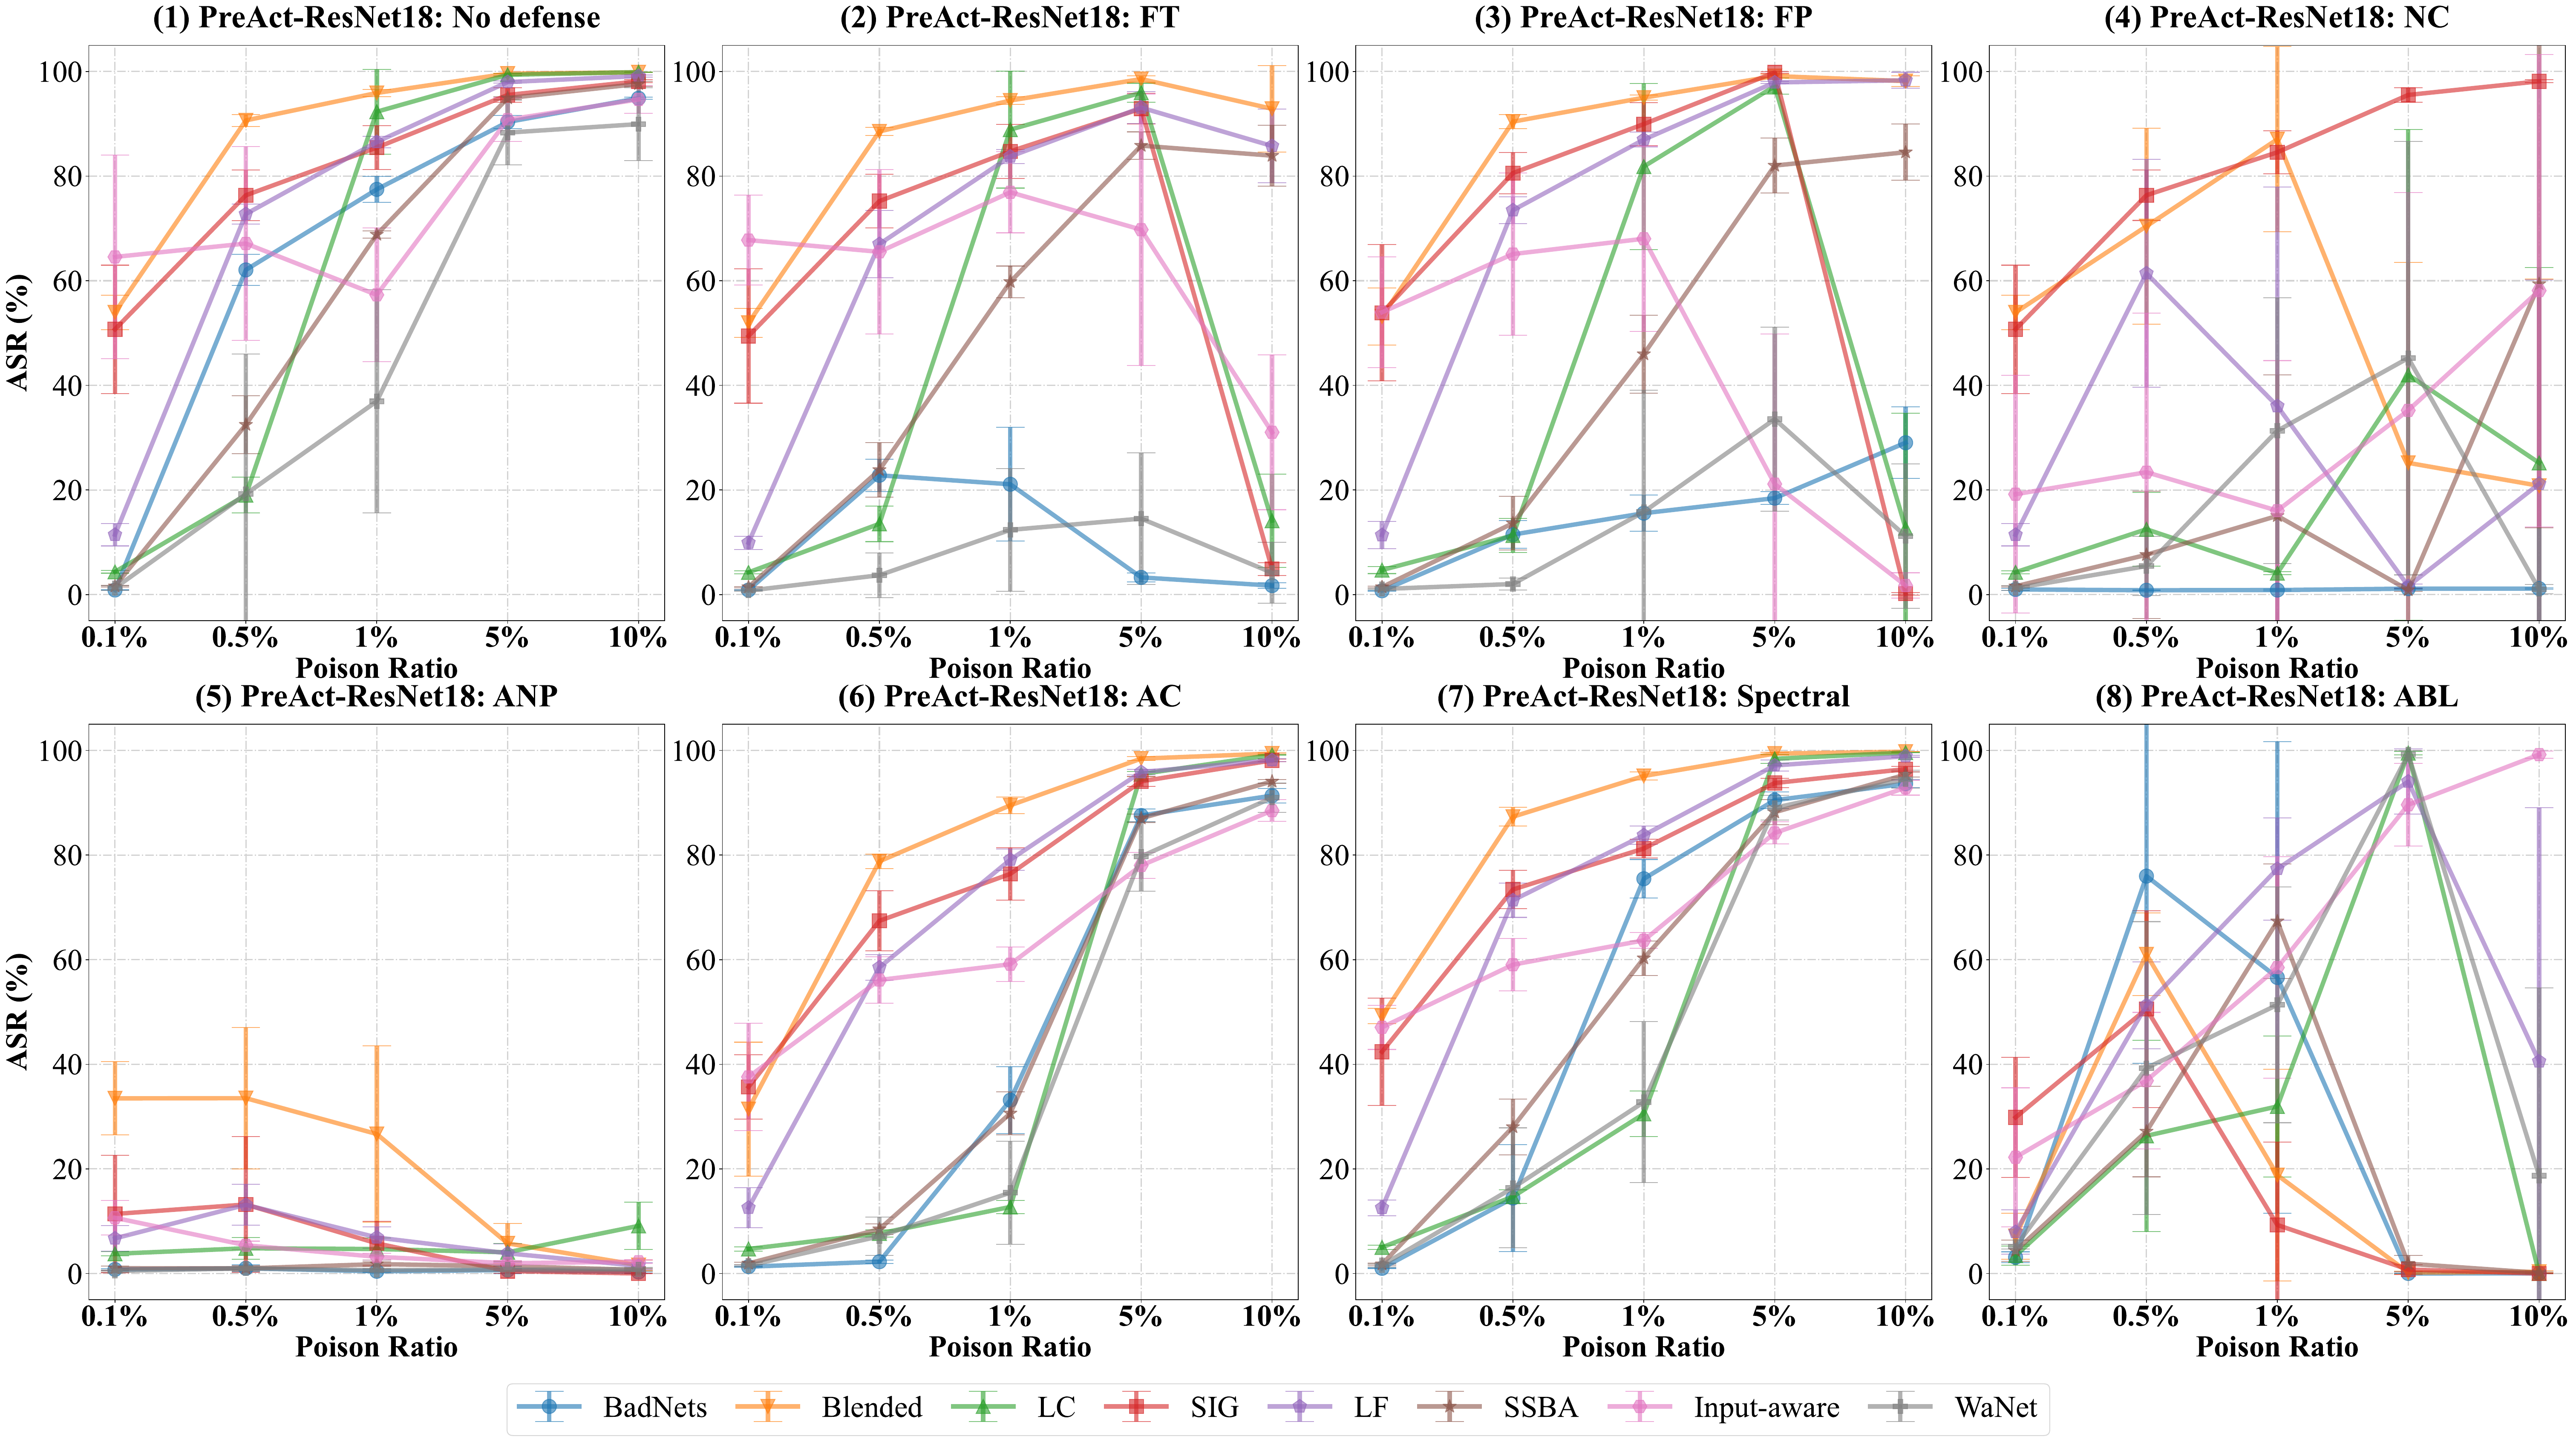}
    % \vspace{-0.7em}
    \caption{\blue{The stability of different poisoning ratios on backdoor learning with 5 random seeds}}
    % \vspace{-1.6em}
    \label{stability-of-poison-ratio}
\end{figure}

\paragraph{Experimental analysis}
\blue{
The trends of ASR curves are generally consistent with those in FIG. \ref{2-attack-asr-preact}, and the error bar is small, indicating that the experimental results are stable. The error bar of ABL is larger when the poisoning ratio is low. ABL identify 1\% of training data as backdoor data with ragard to the training loss. However, the stability of screening results cannot be guaranteed when the poisoning ratio is low. At the same time, we find that there are some differences in the trend of NC method when default parameters are used for attacks against low frequency. In addition, the Error bar of NC is relatively high. NC reversely generates triggers through the backdoor network. The experimental results show that for sample-specific trigger or some large trigger, NC cannot stably judge whether the trigger exists. When NC identifys the similar trigger, the ASR is lower after unlearn, but when NC 
judges it is not a backdoor model through anomaly detection, the trained will maintain the original model with the high ASR, resulting in a large error bar.}
